# Supplementary material for: Grotthuss-type oxygen hole polaron transport in desodiated Na$_{2}$Mn$_3$O$_7$
Source: arXiv:2504.02054 source file (2025-06-16)
Supplement: Supplementary file 1 [file SI.pdf]

**Supplemental Material for: “Grotthuss-type oxygen hole polaron transport in desodiated  $\text{Na}_2\text{Mn}_3\text{O}_7$ ”**

Ming Lei<sup>1,\*</sup>, Iwnetim I. Abate<sup>1,†</sup>

<sup>1</sup>*Department of Materials Science and Engineering, Massachusetts Institute of Technology, Cambridge, MA 02139, USA*

\*mlei012@mit.edu; †iabate@mit.edu

Here we present a set of intermediate structures obtained by linear interpolation of atomic coordinates between the split and 3NN polaron configurations.

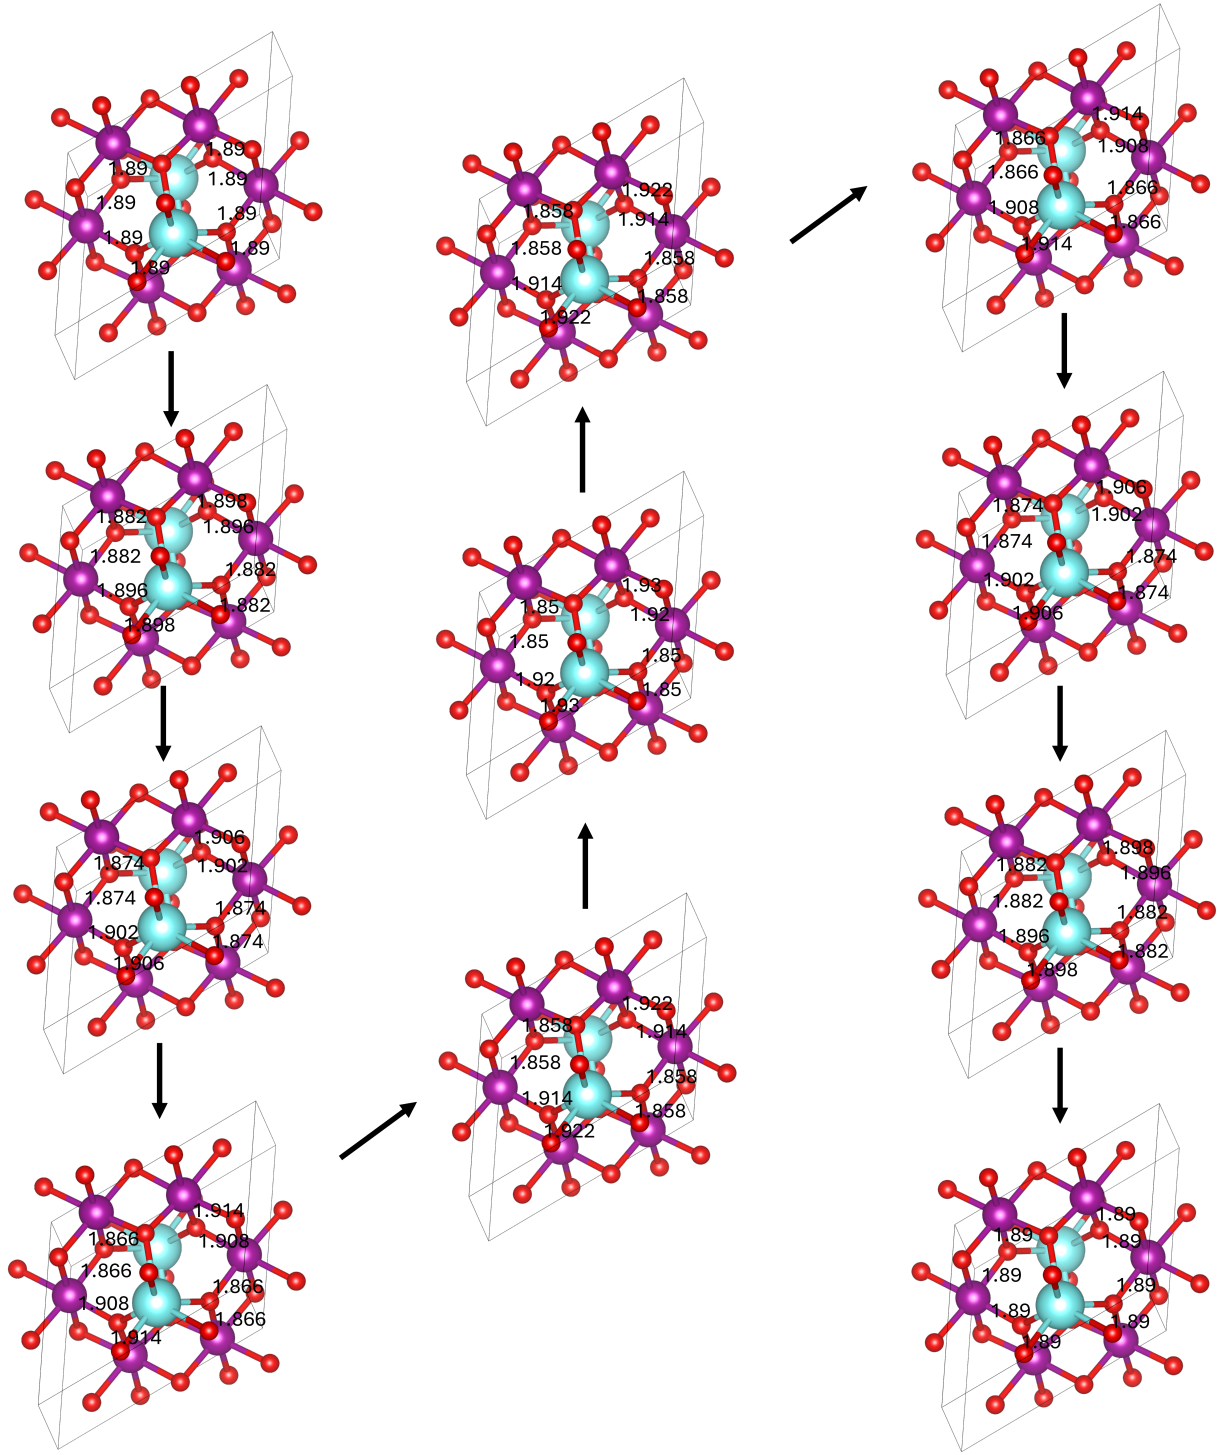

FIG. 1. The intermediate structures obtained by linear interpolation of atomic coordinates between the split and 3NN polaron configurations.
